# Supplementary material for: Improving Non-autoregressive Translation Quality with Pretrained Language Model, Embedding Distillation and Upsampling Strategy for CTC
Source: arXiv:2306.06345 source file (2024-10-14)
Supplement: Supplementary file 1 [file appendix.tex]

\appendix

\section*{Statistics of Datasets} 
\label{sec:static_datasets}
For WMT'14 En$\leftrightarrow$De, the test set is \verb|newstest2014| while we follow \cite{xu-etal-2021-bert} and combine \verb|newstest2012| and \verb|newstest2013| for validation. The statistics of all 3 corpora are summarized in TABLE~\ref{tab:data-static}. We adopt the same preprocessing steps as \cite{gu-kong-2021-fully} for WMT'16 En$\leftrightarrow$Ro and WMT'14 En$\leftrightarrow$De. All the data are tokenized by the Huggingface tokenizer\footnote{\url{https://huggingface.co/docs/transformers/main_classes/tokenizer}} associated with the PMLM.
\input{TABLEs/data-static.tex}

\section*{Knowledge Distillation Teachers Details} \label{sec:KD_details}
For IWSLT'14 En$\leftrightarrow$De, the model configuration for the base transformers is \verb|transformer_iwslt_de_en|, and the strong AT model is the state-of-the-art model proposed by \cite{xu-etal-2021-bert} which is a transformer model of configuration \verb|transformer_iwslt_de_en| (4-512-1024) with a frozen BiBERT model as its contextualized input embeddings. For WMT'14 En$\leftrightarrow$De, the model configurations for the base transformers are \verb|transformer_base| (8-512-2048) and \verb|transformer_vaswani_wmt_en_de_big| (8-1024-4096), and the strong teacher is the same as that of IWSLT'14 En$\leftrightarrow$De except the transformer model's configuration is \verb|transformer_vaswani_wmt_en_de_big|. Note that the scores and distillation data of the BiBERT teacher models on IWSLT'14 En$\leftrightarrow$De and WMT'14 En$\leftrightarrow$De are based on our runs. For WMT'16 En$\leftrightarrow$Ro, the model configuration for the base transformers is \verb|transformer_base|, and the strong teachers are from \cite{bhosale-etal-2020-language}, both of which are trained with back-translation data \footnote{\url{https://data.statmt.org/rsennrich/WMT'16_backtranslations/}}.

\section*{ED with Different Distillation Layer} \label{sec:Different_ED_layer}
 The last layer of each PMLM is chosen for ED in the previous experiments. Here we also explore distilling from other layers and report the performance in Figure \ref{fig:Pretrained Model and KD-M Layer}. The performance of each layer is relatively consistent in the BiBERT model, except the ninth layer is slightly lower than others. Distilling from the tenth layer has the best performance with mBERT model, and distilling from any layer is better than without distilling in the IM setting. IM is better than IT, except for no ED for mBERT.
\begin{figure}[h]
    \centering
    \includegraphics[width=0.45\textwidth]{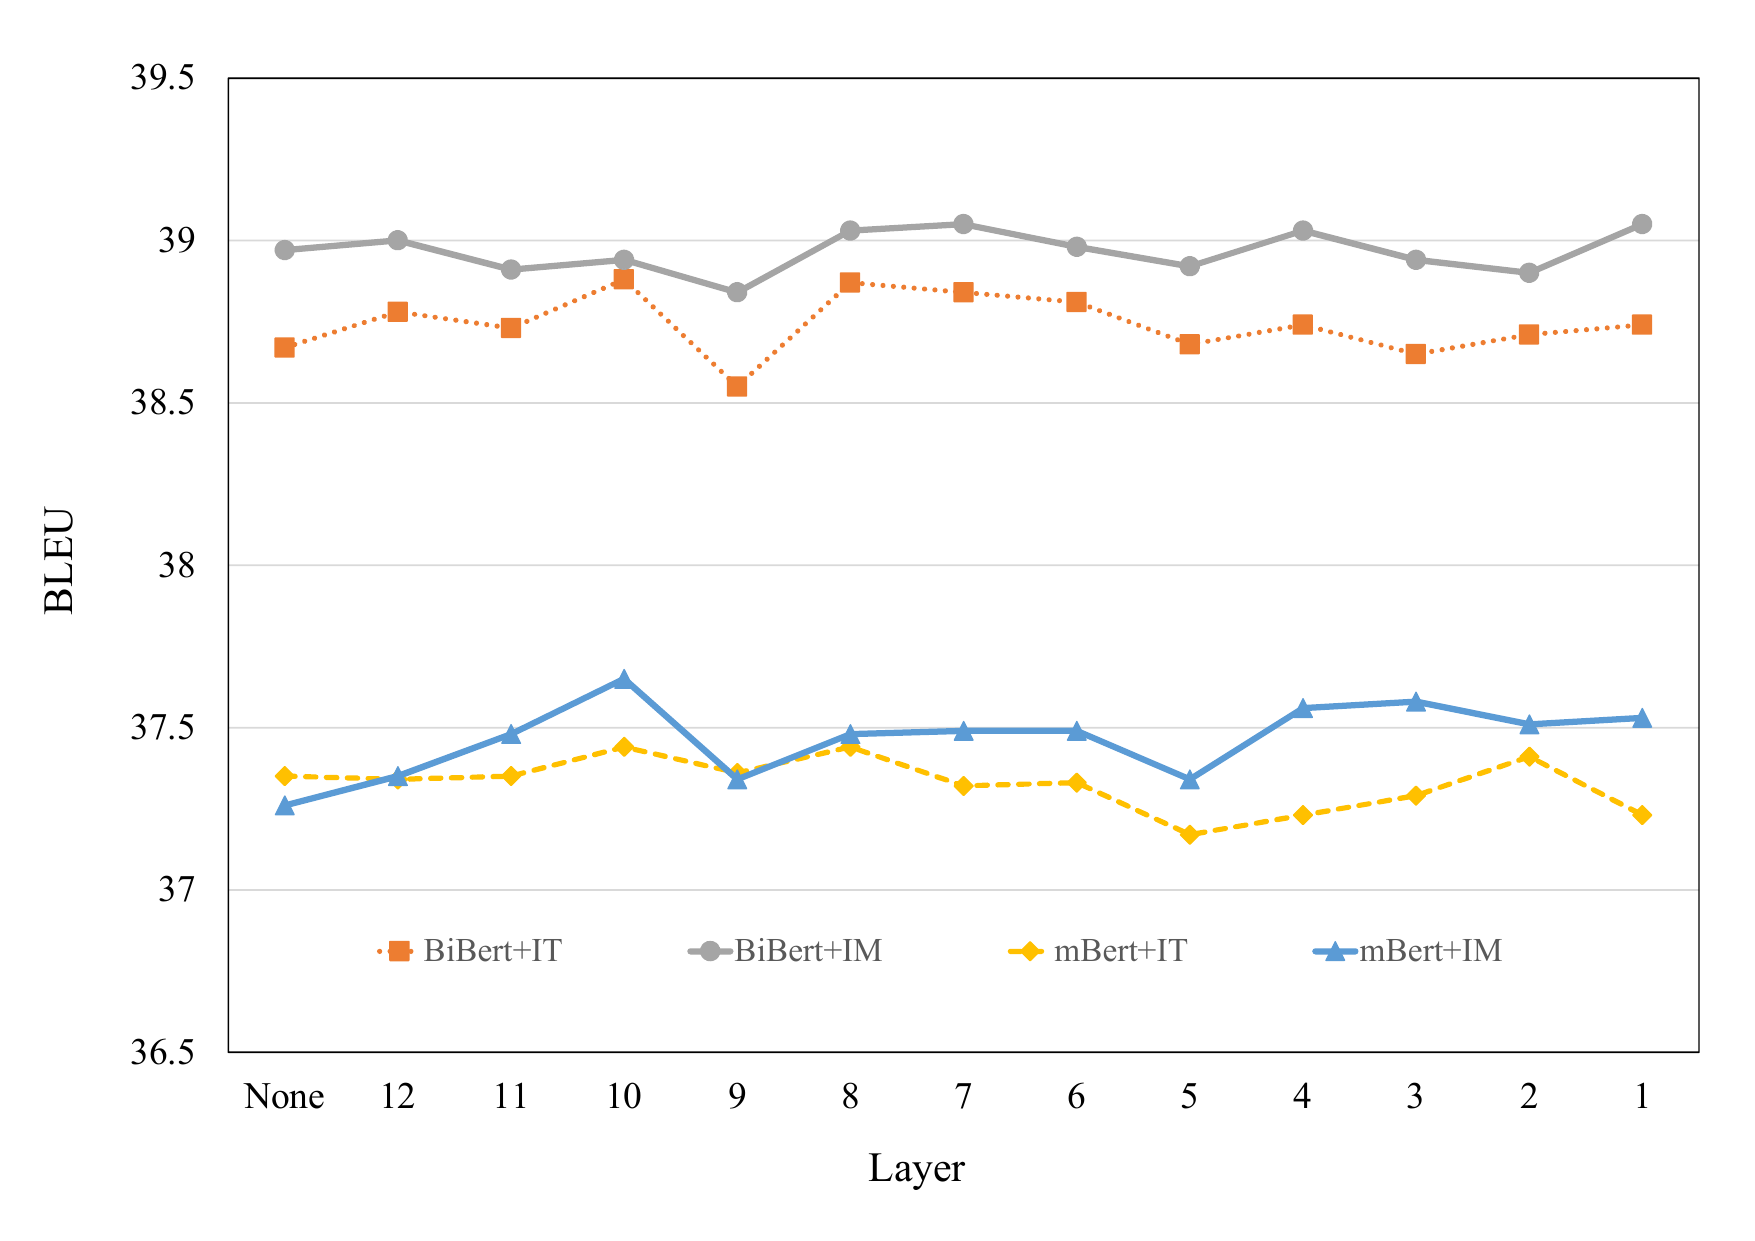}
    \caption{BLEU v.s. Distillation Layer on the test set of IWSLT'14 DE$\rightarrow$EN. We compare different distillation layer on BiBERT and mBERT respectively, with upsampling ratio $s=2$ and FR. Here "None" means not using ED method.}
    \label{fig:Pretrained Model and KD-M Layer}
\end{figure}

\section*{Training Details} \label{sec:train_details}
 For our NAT models, the dropout rates are all 0.1 and learning rates are all $10^{-4}$. For IWSLT'14 En$\leftrightarrow$De, the NAT models are trained with 12.8k tokens in a batch for 100K updates. For WMT'16 Ro$\leftrightarrow$En the NAT models are trained with 65K token in a batch for 30K updates. For WMT'14 En$\leftrightarrow$De the NAT models are trained with 65k tokens in a batch for 100K update. The $\lambda$ in equation \ref{eqn:lctc} is set to 0 for the first 75k steps and then to 1 for the remaining steps on both IWSLT'14 En$\leftrightarrow$De and WMT'14 En$\leftrightarrow$De. As for WMT'16 Ro$\leftrightarrow$En, the $\lambda$ is set 0 for the first 20k steps and then to 1 for the remaining steps. We analyze the training cost on three datasets, and the result is show in TABLE~\ref{tab:train-cost}.\\
 In TABLE~\ref{tab:ed-training}, we also include a comparison between using ED and not using ED, specifically for an upsampling rate of $s=4$, which is our best setting. The models were trained on 4 Nvidia-3090-GPUs for 100k steps on IWSLT'14 En$\leftrightarrow$De dataset.
 
\input{TABLEs/train-cost.tex}
\input{TABLEs/ed-training.tex}

%  \section{Different Model} \label{sec:Different_Model}
%  In addition to the BiBERT and mBERT in the previous sections, we also compared other pretrained multilingual models (PMLMs), such as DistilBERT\footnote{\url{https://huggingface.co/distilbert-base-uncased}}(\verb|distilbert-base-uncased|) and XLMR\footnote{\url{https://huggingface.co/xlm-roberta-base}} (\verb|xlm-roberta-base|), and the results are shown in the TABLE~\ref{tab:diff_pmlm}. The model achieves better accuracy by initializing with BiBERT PMLM, which may be due to that BiBERT is pre-trained only on German and English and thus has more consistent alignment between the tokens of both languages. Additionally, XLMR achieves the best performance among PMLMs with more than three languages, but it requires more parameters and has lower inference speed. 
% \input{TABLEs/pmlms}
